# Supplementary material for: Forced imbibition in porous media: a fourfold scenario
Source: arXiv:1705.07775 ancillary file (2017-05-22)
Supplement: Supplementary file 1 [file Supplementary.pdf]

# Forced imbibition in porous media: a fourfold scenario.
# Supplementary informations

Céleste Odier,[1,2] Bertrand Levaché,[2,3] Enric Santanach-Carreras,[2,3] and Denis Bartolo[1]

[1] *Univ Lyon, Ens de Lyon, Univ Claude Bernard, CNRS, Laboratoire de Physique, F-69342 Lyon, France*

[2] *Total SA. Pôle d'Etudes et Recherche de Lacq, BP 47-64170 Lacq, France*

[3] *Laboratoire Physico-Chimie des Interfaces Complexes, Total-ESPCI Paris-CNRS-UPMC, BP 47-64170 Lacq, France*

## CONTENTS

I. Experiments 1
  A. Microfluidics 1
  B. Measure of the local film thickness from light absorption 2
  C. Roughness of the sticker surface: AFM measurements 2

II. Imbibition transitions observed upon increasing the viscosity ratio 2

III. Description of the Supplementary Movies 4
  A. Supplementary Movie 1 4
  B. Supplementary Movie 2 4
  C. Supplementary Movie 3 5
  D. Supplementary Movie 4 5
  E. Supplementary Movie 5 5

References 5

## I. EXPERIMENTS

### A. Microfluidics

The experiment consists in injecting an aqueous solution in a microfluidic porous medium filled with silicon oil (Bluesil 43V Oils of viscosity ranging from 5 cp to 3500 cp). The aqueous solution is a mixture of water, SDS (1 wt%) and food dye (0.2 wt%) for light-absorption experiments. The food dye is replaced by 0.02 wt% of fluorescein for confocal imaging experiments.

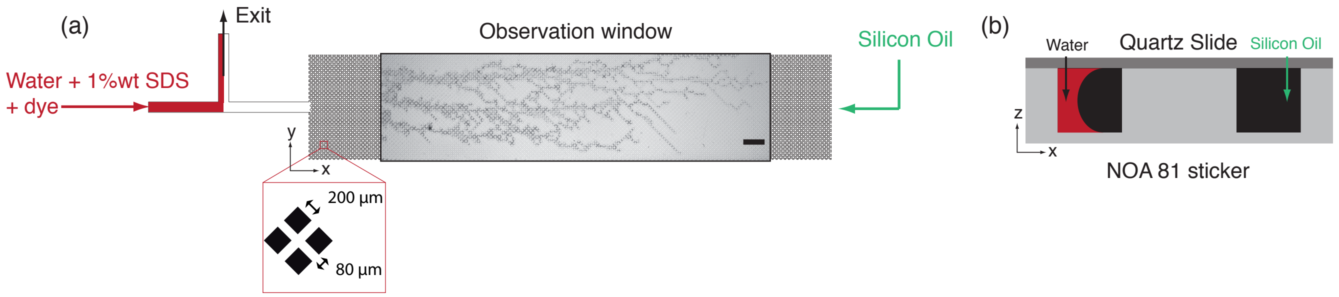


Figure S1. (a) Sketch of the microfluidic channels, and of the initial shape of the water-silicon oil interface with a zoom on the local geometry. The observation window is represented by a typical image corresponding to regime C. The porous medium is filled with silicon oil (transparent) displaced by the colored aqueous solution forming a river-network pattern. Scale bar 2 mm. (b) Sketch of the geometry in the transverse plane.

The channels are made by bonding a micro-patterned sticker to a Quartz slide as described in [1]. The sticker is made by imprinting a thin film of thiolene-based resin (NOA 81, Norland Optical Adhesives) on a glass coverslip

with a PDMS stamp patterned with the desired channel geometry. The sticker is then sealed with a Quartz slide by means of UV exposure and thermal curing (12 h at 90°). The four walls of the channels are then made hydrophilic by *in situ* UV treatment (deep-UV exposure for 30 mins, Jelight UVO Cleaner 42) as thoroughly described in [2]. The geometry of the resulting channels is shown in Fig. S1. The channel height is constant over the entire device, $H = 70 \pm 2\,\mu$m, and does not change as the fluids are flown. The width and the length of the main channel including the porous medium are $W = 1$ cm, and $L = 5$ cm respectively. The porous medium is a square lattice of 200 $\mu$m-wide square posts separated by 80 $\mu$m-wide channels .

In order to ensure reproducible initial conditions, the devices are filled following a systematic sequence of injection steps. First, the channel is filled with silicon oil by applying a constant 100 mbar pressure which is kept constant over the entire experiment. Then, the aqueous solution is flown at constant flow rate with a precision syringe pump (Nemesys, Cetoni). The two fluids meet at a T-junction and form a flat interface, Figure S1. Once the interface reaches a stationary shape, the T-junction outlet is closed which triggers the invasion of the porous medium by the aqueous solution. In order to avoid any possible modification of the wetting properties of the hydrophilic surfaces by the adsorption of water, surfactant, or dye molecules, the chips are *not* recycled. The data reported in the main text correspond to experiments performed in more than a hundred different devices.

### B. Measure of the local film thickness from light absorption

The invasion patterns are observed with a 60 mm macro lens (Nikkor f/2.8G, Nikon) mounted on a 8 Mpxls, 14bit CCD camera (Prosilica GX3300). The resulting spatial resolution is 11 $\mu$m/pxl. We convert the transmitted-light intensity into the local water-pattern thickness with an estimated relative precision of 1 $\mu$m. The local thickness $h(x, y, t)$ of the water films relates to the image intensity $I(x, y, t)$ via the Beer-Lambert absorption law:

$$h(x, y, t) = -\epsilon c \ln \frac{I(x, y, t)}{I_0(x, y, t)} \tag{1}$$

where $c_0$ is the dye concentration, $\epsilon$ is the absorptivity, and $I_0$ is the transmitted intensity for a channel filled with silicon oil. The coefficient $\epsilon$ was determined by performing experiments with colored water only, in step channels of known height using solutions of increasing concentrations as illustrated in Figs. S2a and S2b. The excellent agreement between the thickness measured from the transmitted light intensity and the nominal depth of the step channel is shown in Fig. S2c. The spatial dispersion of the height field is smaller than 4 $\mu$m (error bars in Fig. S2c). This dispersion results from the combination of the mold heterogeneities and of the intrinsic limitation of the measurement method.

The performance of the local height measurement is better illustrated by a direct measure of the surface heterogeneities of the primary mold used to imprint the sticker. The step channel is made by micro-milling Plexiglas (CNC MicroMill, Minitech Machinery). Replicating the mold with PDMS and looking at a transverse cut tells us about the (small) roughness of the surface, see Fig. S2b. The small bumps shown by the arrows in Fig. S2b correspond to the path of the mill. These minute irregularities of the mold are seen very clearly on the height profile measured by light-intensity measurements in Fig. S2c.

Note that the measure of $I_0(x, y)$ allowed us to correct the spatial heterogeneities of the observation setup. We also performed a systematic correction of the temporal fluctuations of the light source by bringing the average light intensity outside the channel to the same value for all images.

### C. Roughness of the sticker surface: AFM measurements

In order to measure the roughness of the sticker surfaces, we prepared samples with the same protocol as for actual experiments using flat PDMS stamps (replica of a silicon-wafer surface). The topography of the surface is measured with an Atomic Force Microscope, see Fig.S3, in a Multimode 8 system, with Nanoscope V controller (Bruker), operated in Tapping mode in air with a RTESP300 cantilever (Bruker) characterized by a typical spring constant $k = 40$ N/m and tip radius $R = 5$ nm. The surface roughness defined as the standard deviation of the local height field is $\sigma_Z = 8.3$ nm.

## II. IMBIBITION TRANSITIONS OBSERVED UPON INCREASING THE VISCOSITY RATIO

We now report experiments where we mobilized oils of increasing viscosities while keeping the capillary number $Ca = 2.2 \times 10^{-4}$ constant. The geometry of the device is locally the same as in the main text (square post of width

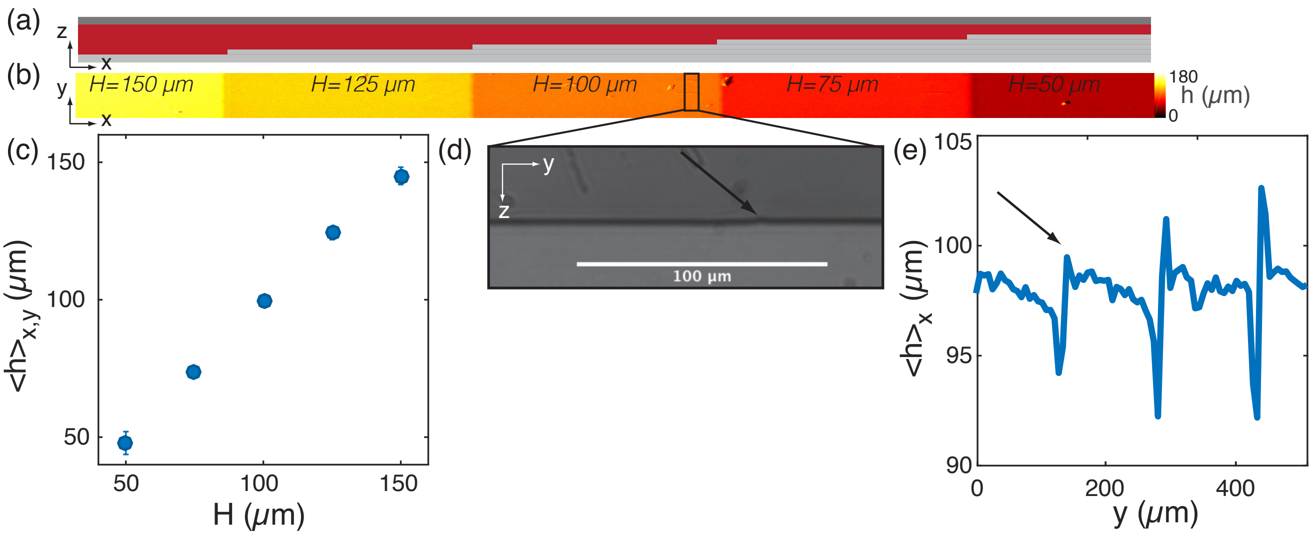


Figure S2. Benchmark of the film-thickness measurement. (a) Sketch of the step-channel geometry. (b) Water thickness measured in the step channel with known concentration of dye. (c) Evolution of the measured thickness with the height of the step mold. The average is taken over regions of 1 mm × 3 mm. Error bars 1$\sigma$. (d) Cut of the PDMS mold used to imprint the microfluidic channel. The cut corresponds to the black rectangle in (b). (e) Profile of the mean thickness averaged over 500 $\mu$m along the $x$ direction. The two arrows indicate the peaks corresponding to the bumps hardly visible in (d).

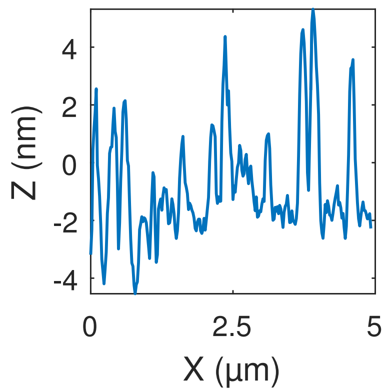


Figure S3. Topography of the sticker surface measured by Atomic Force Microscopy. Example of height variations measured along a 5 $\mu$m line.

200 $\mu$m) but the overall dimensions of the porous medium are here 4 cm × 1.5 cm. In Fig. S4a we show the imbibition patterns at percolation obtained for eight different viscosity ratios.

Regime A: For $M < 22$ we observe the classical capillary imbibition regime referred to as regime A in the main text. Water fills the entire gap of the channels, and the macroscopic pattern reflects the underlying square geometry. We note that increasing $M$ results in the formation of narrower fingers.

Regime B: For $M > 22$, we observe the characteristic patterns of Regime B, heterogeneous films form a fingering pattern with a number of fingers increasing with $M$.

Regime C: The transition from regime B to regime C occurs for $28 < M < 50$. It is less sharp than that reported in the main text. For $M = 33$, we do not observe droplets trapped at the vertices of the lattice, but some snap-off events are locally observed. Locally the flow does not fully stabilize the water-film interfaces. Above $M = 50$, both the microscopic dynamics and the large-scale patterns are unambiguously typical of regime C. We also note that increasing $M$ results in increasingly thin rivers.

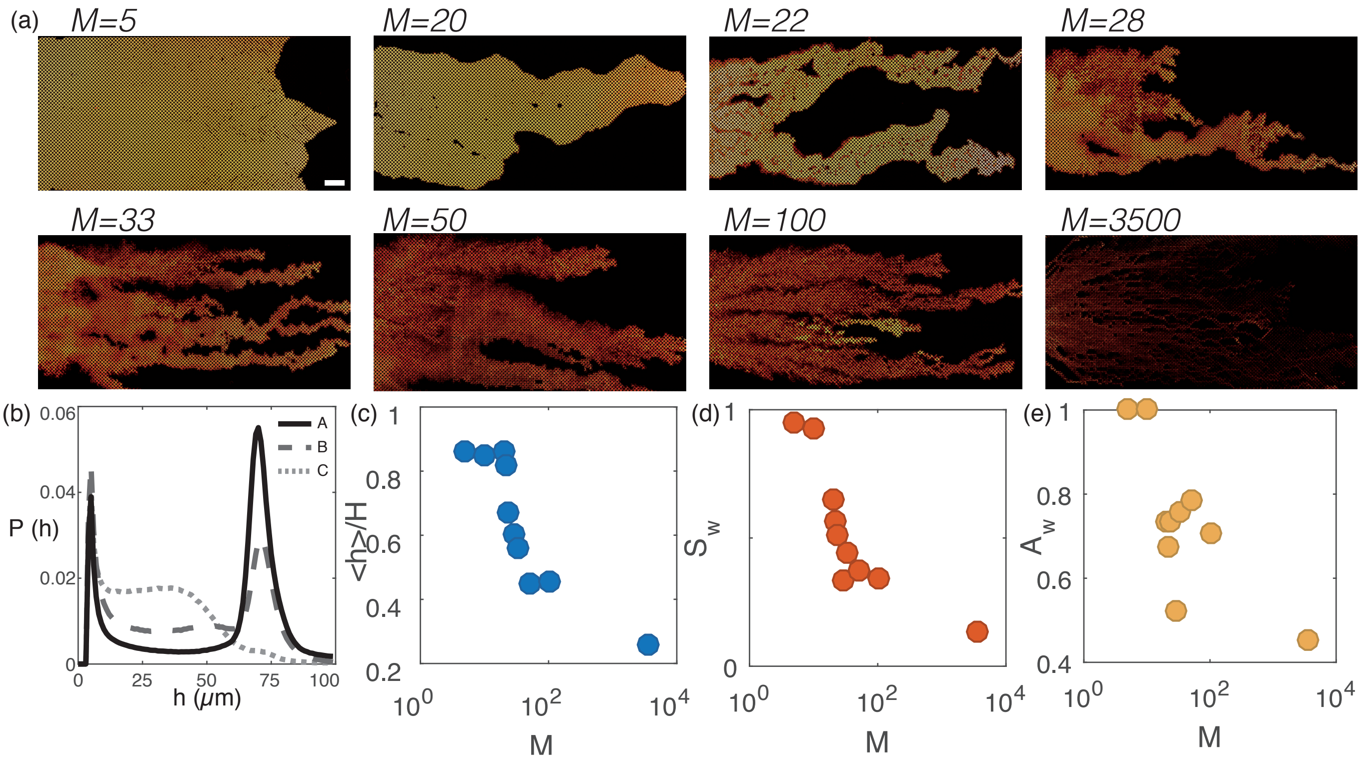


Figure S4. Imbibition patterns. (a) Eight imbibition patterns at different viscosity ratio. Scale bar 2 mm. (b) Probability distribution of the local water-film thickness for $M = 5$ (regime A), $M = 23$ (regime B) and $M = 100$ (regime C). (c) Average thickness of the water films normalized by the average height of the channels. (d) Variations of the water saturation with $M$. (e) Variations of the wetted area fraction with $M$.

No regime D: Increasing the viscosity ratio up to values as large as $M = 3500$, we did not observe any sign of reversal of the apparent contact angle and of the entrainment transition typical of Regime D. Instead, extremely thin water films still progress along the solid surfaces.

More quantitatively, regimes A, B and C are clearly distinguished on the PDF of the local film thickness, Fig. S4b. In agreement with the related discussion in the main text. The transition between regimes A and B occurs as the relative magnitude of the peaks at $h = 0$ and $h = H$ exceeds one. The transition between regime B and C translates into the suppression of the peak at $h = H$ and a PDF with an extended flat region preventing the identification of a typical film thickness. The mean thickness ($\langle h \rangle$), of the water saturation ($S_{\rm w}$) and of the wetted area fraction ($A_{\rm w}$) are monotonically decreasing functions of the viscosity ratio. The higher the oil viscosity the lower the recovery rate.

## III. DESCRIPTION OF THE SUPPLEMENTARY MOVIES

### A. Supplementary Movie 1

Movie showing four imbibition patterns corresponding to the four regimes discussed in the main text and presented in Fig. 1a. The color indicates the local thickness of the water films.

### B. Supplementary Movie 2

Movie showing the four dynamical regimes at the pore-scale presented in Fig. 2a. The color indicates the local thickness of the water films.

### C. Supplementary Movie 3

Confocal images of the interface propagation in the $xy$ plane, 5 $\mu$m above the sticker surface in Regime B (Fig. 2b). $Ca = 7 \times 10^{-5}$, $M = 560$.

### D. Supplementary Movie 4

Movie showing the destabilization of the thin films (Regime C) after an abrupt stop of the flow. Oil droplets form and are trapped at the vertices of the network when the flow stops (see also Fig. 2e). $Ca = 2.2 \times 10^{-4}$, $M = 560$.

### E. Supplementary Movie 5

Evolution of the imbibition pattern in regime C (Fig. 3a in the main text). The thin films coarsen. The color indicates the local height of the water films. $Ca = 5 \times 10^{-4}$, $M = 560$.

[1] Denis Bartolo, Guillaume Degre, Philippe Nghe, and Vincent Studer, "Microfluidic stickers," Lab Chip **8**, 274–279 (2008).
[2] Bertrand Levache, Ammar Azioune, Maurice Bourrel, Vincent Studer, and Denis Bartolo, "Engineering the surface properties of microfluidic stickers," Lab Chip **12**, 3028–3031 (2012).
